# Supplementary material for: Enabling High-Quality In-the-Wild Imaging from Severely Aberrated Metalens Bursts
Source: arXiv:2510.10083 source file (2025-10-11)
Supplement: Supplementary file 1 [file ablations.tex]

\section{Discussion on Ablation studies}

Table 4 of the main paper we explore the contribution of each individual component to the overall performance of the restoration pipeline. From the reported metrics the following observations can be made:

\begin{enumerate}[label=\textbf{\roman*}, leftmargin=*]
\setlength{\itemindent}{0em}
    \item \textbf{Increasing number of burst frames:} Increasing the number of burst frames had a strong effect in the performance for the BAFN module which improves due to better noise averaging and information redundancy. However, the weight branch does not observe a similar trend. This can be owed to the limited flexibility of the weight branch with only a few learnable paramaters compared to the BAFN module.
    \item \textbf{Channel Depth:} Increasing channel depth improves the PSNR metric significantly from 24.3 to 26.5 when moving from channel size of 16 to 24 but further improvements are not observed when increasing to 32.
    \item \textbf{Burst attention units:} Increasing the number of self attention units helps improve performance but improvements with more burst attention units saturates after a point.
    % \item \textbf{:} We observe that one of our most impactful additions to the ControlNet architecture is using the MLCN instead of a linear encoder chain and using a NAFBlock \cite{chen2022nafnet} instead of the simple convolutional encoder used in the original architecture. We record an increase in all 3 metrics PSNR, SSIM and LPIPS when using this combination.
    % \item \textbf{Curriculum training process:} Finally, the curriculum learning schedule also provides a notable boost in terms of SSIM due to its stable training process.
\end{enumerate}
