# Supplementary material for: Enabling High-Quality In-the-Wild Imaging from Severely Aberrated Metalens Bursts
Source: arXiv:2510.10083 source file (2025-10-11)
Supplement: Supplementary file 2 [file intro.tex]

We organize the supplementary document into 3 sections namely, the camera design, additional implementation details and additional results and figures.

\section{Camera design} 
\begin{figure*}[!htbp]
    \centering
    \includegraphics[width=\linewidth]{figures/assets/SEM_image_CVPR.png}
    % \vspace{-4mm}
    \caption{Meta-atoms visible under an electron microscope}
    \label{fig:meta_fab}
\end{figure*}

\subsection{Metalens Optimization} 
% As explained in the main text, we optimized the metalens phase profile $\phi(r)$ 

% \subsection{Metalens Phase Function Optimization}
Metalenses are flat optical devices that focus light using arrays of nanoscale antennas rather than curved surfaces. Each antenna imparts a precise phase delay to create the desired optical function through controlled interference.
Nanostructures provide discrete phase values, performance varies with wavelength and incident angle, and manufacturing imposes geometric limitations. These factors prevent direct implementation of ideal phase functions which ordinary refractive lenses such as convex lenses follow.
Modern approaches use differentiable wave propagation models for end-to-end optimization. Light propagation from metalens to the image plane can be simulated using differentiable operations such as Fast Fourier Transforms. Phase parameters ($\phi(r)$) are iteratively optimized using gradient descent to minimize optical performance metrics such as focal spot size or aberration levels.
This computational approach helps us design complex optical functions that exceed traditional lens capabilities while addressing practical manufacturing and performance constraints.

\subsection{Metalens Fabrication and Assembly}
We fabricated a 1 cm large aperture metaoptic using a nanofabrication approach, facilitated
in an ISO Class 5-7 clean room environment. First, quartz
wafer (purchases from University Wafer), were cleaned in
subsequent ultrasonicating baths of Acetone, IPA, and DI
water, then exposed to a short oxygen descum in a Barrel
Etcher. We then deposited an 
$\tilde{}$ 800 nm thick Silicon Nitride
film using plasma enhanced chemical vapor deposition in
an SPTS chamber. Afterwards the wafer was diced into 1.5
cm square pieces and again cleaned using an ultrasonicating
bath and barrel etch steps (as before). We then applied a
positive resist (ZEP 520A) with a thickness of 400nm. To
mitigate charging during the patterning, we also applied a
conductive polymer layer (DisCharge H2O). We then patterned the resist using a 8 nA, 100 keV electron beam (JEOL
JBX6300FS) at a dose of about 300 $\mu C$ $cm^2$. After electron beam lithography, we removed the conductive polymer
layer using a short IPA bath and developed the resist at room
temperature in Amyl Acetate for 2 min. Subsequently, the
sample was again descummed in a short barrel etch step
and a layer of about 75 nm alumina was evaporated onto
the sample. The resist was then lifted off overnight in an
NMP bath at on a hot plate. Subsequently, the SiN layer was
etched using a fluorine based etch mixture in an inductively
coupled reactive ion etcher (Oxford PlasmaLab System 100).
Finally, the chip was integrated in a 3D printed holder and
mounted with the sensor. Scanning Electron Microscope
Images after fabrication can be seen in \cref{fig:meta_fab}. The resulting transmissive metalens is integrated with an Allied Vision 1800 U-510 CMOS sensor and paired with a Jetson Nano Orin board for handheld operation.

% \subsection{Metalens optimization} 

\section{Additional implementation details}

\paragraph{Reference frame selector}  Please refer to the reference selection algorithm pseudo-code in \cref{algo:reference_selection}.
\begin{algorithm}[htbp]
\small
\caption{Reference Frame Selection Algorithm}
\label{algo:reference_selection}
\SetAlgoLined
\KwIn{Reference exposure time $\leftarrow$ ISP, burst size $N$}
\KwOut{Reference frame $I_{ref}$}

$t_{ref} \leftarrow$ AutoExposure()\;
Initialize burst set $\mathcal{B} \leftarrow \{\}$\;

\For{$i = 1$ \KwTo $N$}{
    $g_i \leftarrow$ SampleDigitalGain()\;
    $I_i \leftarrow$ Capture($t_{ref}$, $g_i$)\;
    $\mathcal{B} \leftarrow \mathcal{B} \cup \{I_i\}$\;
}

$s_{max} \leftarrow 0$, $I_{ref} \leftarrow \text{null}$\;

\For{each $I_i \in \mathcal{B}$}{
    $G_i \leftarrow$ ExtractGreenChannel($I_i$)\;
    $s_i \leftarrow$ GradientSharpness($G_i$)\;
    \If{$s_i > s_{max}$}{
        $s_{max} \leftarrow s_i$, $I_{ref} \leftarrow I_i$\;
    }
}
\Return $I_{ref}$\;
\end{algorithm}

\begin{algorithm}[htbp]  
\small  
\caption{Multi-scale Feature Extraction and Homography Estimation}  
\label{alg:multi_homography_part1}  
\SetAlgoLined  
\KwIn{Burst images $\{I^i\}$, deconvolution parameter $\rho$, weights $\{\lambda_k\}$, pyramid levels $K$}  
\KwOut{Homographies $\{H^k\}$ across scales}  

\For{$k = 2$ \KwTo $K$}{  
    Compute $\widetilde{I}^b_k$ via Tikhonov deconvolution:
    
    \[
    \widetilde{I}^b_k = \mathcal{F}^{-1} \left\{ \frac{\bar{\rho^*}}{\lvert\bar{\rho}^2\rvert + \lambda } \mathcal{F}(\widetilde{I}^b_{k-1} \downarrow_2) \right\}
    \]
    where, $\bar{\rho}$ is the optical transfer function or the Discrete Fourier Transform of the PSF ($\rho$) and $\mathcal{F}$  represents the Fast Fourier operation
}  

\For{$k = K$ \KwTo $1$}{  
    Extract feature correspondences and estimate homography:  
    \[
    H^k = \mathtt{get\_pts}(\widetilde{I}^i_k, \widetilde{I}^{i+1}_k)
    \]  
}  
\end{algorithm}

\begin{algorithm}[htbp]  
\small
\caption{Multi-scale displacement fusion}
% \caption{Compute $\{\vec{V}_p\}_K^i$ from homography $H^K$ and Hierarchical Refinement}  
\label{alg:multi_homography_part2}  
\SetAlgoLined  
\KwIn{Homographies $\{H^k\}$, pyramid levels $K$}  
\KwOut{Displacement maps $\{\vec{V}_p\}_i^b$ (final aligned flow fields)}  

Initialize global displacement from coarsest level:  
\[
\{\vec{V}_p\}_K^i \quad \text{from } H^K
\]  

\For{$k = K-1$ \KwTo $1$}{  
    \For{each patch $p$}{  
        Compute local homography $H_p^k$ and displacement $\{\vec{V}_p\}_k^i$  

        Fix the weight to a constant value:  
        \[
        \omega_p = 0.5 \quad \text{(empirically chosen constant)}
        \]  

        Update displacement via weighted aggregation:  
        \[
        \vec{V_p}_k^i = (1 -\omega_p)\,\mathtt{best}\bigl(\vec{V_p}_k^i, 
        \:\:\:\: \{\vec{V_{p'}}_k^i\}_{p' \in \mathcal{N}(p)}\bigr) + \omega_p \,\vec{V_p}_{k+1}^i
        \]  
    }  
}  
\end{algorithm}

\paragraph{Multi-scale burst alignment algorithm} Similar to HDR+, our method also adopts a pyramid-based iterative refinement strategy for displacement estimation. As shown in \cref{fig:rebut_multi}, however, under the same framework our multi-scale displacement fusion produces motion fields that are notably more coherent and stable across pyramid levels. The displacement map indicates a pronounced shift in the upper-left and only subtle motion in the bottom-right (with the red object nearly static), all of which are faithfully captured by our flow visualization. In contrast, HDR+ \cite{hasinoff2016burst} provides reasonable estimates in the upper-right and red object regions but substantially overestimates motion in the bottom-right, yielding incorrect magnitudes and directions. Our method, on the other hand, preserves smooth global motion patterns and structural consistency, leading to more reliable alignment. Moreover, in the bottom-left region our flow reveals a clear downward displacement, not evident in the displacement map due to the repetitive vertical texture of the floor tiles, demonstrating the robustness of our approach for burst imaging with complex textures and weak motions.The complete pseudo-code is detailed in \cref{alg:multi_homography_part1,alg:multi_homography_part2}.

\begin{figure}[t]
    \centering
    \includegraphics[width=\linewidth]{figures/assets/fig_rebut1_2_multi.pdf}
      \caption{\textit{Multi-scale displacement fusion.} The first row shows the reference frame, target frame, and their displacement map. The subsequent rows visualize flow fields across pyramid levels (k = 0, 1, 2), where arrow direction encodes motion direction and arrow length/color encode displacement magnitude.}
    \label{fig:rebut_multi}
    % \vspace{-2mm}
\end{figure}

\paragraph{Adaptive pixel correction unit (APCU)} The adaptive pixel correction unit is designed similar to the weighted burst fusion block using a series of residual blocks followed by a sigmoid weighting layer,
\begin{equation}
    \label{eq:apcu}
I_\text{init} = I_\text{fused} \cdot \mathtt{sigmoid}(\{\mathtt{ResBlocks}^n(I_\text{fused})\})
\end{equation}

\paragraph{Attention Fusion Block}

The skip connections from the SFT layer, containing features for all burst frames, are fused into the attention fusion block (AFB). Fusion between the reference and other burst frames is modeled using a series of channel-wise cross-attentions:
\begin{align}
    \mathtt{AFB}(\{SFT\}_i) &= \mathtt{crossatten}(CA^{n}, \{SFT\}_i - SFT_\text{ref})\nonumber\\
    CA^{n} &= \mathtt{crossatten}(CA^{n-1}, \{SFT\}_i - SFT_\text{ref})\nonumber\\
    CA^0 &= SFT_\text{ref}\nonumber
\end{align}
where $SFT_\text{ref}$ is the scale-shift features coming from the skip connections for the reference frame index and cross-attention is performed via multi-head attention (MHA) between the query ($CA^n$) and all the burst frames as the context:
\begin{align}
    \mathtt{crossatten}(Q, \{SFT\}_i) &= \{\mathtt{MHA}(Q^h, K^h, V^h)\}_b\nonumber\\
    Q^h = f^h_q(Q), K^h &= f^h_k(SFT_i), V^h = f^h_v(SFT_i) \nonumber
\end{align}
where $\mathtt{MHA}$ denotes multi-head attention over heads $h$, and $f^h_{(.)}$ are depthwise separable convolutions. The resulting value $D$ is then added to $SFT_{ref}$ and forwarded to the U-net decoder,
\begin{equation}
    D = \mathtt{AFB}(\{SFT_i\}) + SFT_\text{ref}.\nonumber
\end{equation}

\textbf{Unsupervised finetuning} For real-world adaptation, we perform fine-tuning using the saturation loss $L_{sat}$ computed on saturation masks. We reduce the learning rate by a factor of 10 from the base model's training rate and freeze all model layers except the fusion weight prediction network. The weight prediction network parameters are updated using an exponentially moving average with decay factor 0.995 across iterations. We also include the original training losses computed over a small subset of synthetic training data during fine-tuning. The saturation loss on real images and original training losses on synthetic images are balanced by a weighting factor determined through cross-validation. Fine-tuning continues until the combined loss converges and no longer decreases.

\section{Additional results and ablations} 
\subsection{Additional results}
We provide evaluation results of our burst restoration framework on OLED dataset in \cref{figure:comp_1080}, showing superior image quality and restoration of finer details. In \cref{tab:bmatch_2}, we show further evaluations of our burst alignment algorithm at different exposure levels and more visual comparisons in \cref{fig:di_supp}. In \cref{fig:real_images_sup} we provide visual results for in-the-wild restoration without any manual intervention during the capture process. As shown in the figure, our method can generalize under arbitrary lighting conditions due to our robust training strategy. As an added bonus our in-the-wild adaptation in Sec. 4.4 helps generalize to outdoor HDR scenes as shown in \cref{fig:hdr_supp}. We analyze exposure fusion maps from the burst fusion module in \cref{fig:expmap_sup} and compare against those of Mertens et al. \cite{mertens2007exposure}. We also separately show in \cref{fig:I} the contribution of the restoration module ($I_\text{res}$) from the modules before it ($I_\text{init}$).

\begin{table}[h!]
\centering
\caption{MetaHDR Dataset Composition}
\setlength{\tabcolsep}{4pt}

\begin{tabular}{@{}cccp{2cm}c@{}}
\toprule
\textbf{Dataset} & \textbf{Size} & \textbf{\#Burst} & \textbf{Scenes} & \textbf{Train\%} \\
\midrule
\multicolumn{5}{l}{\textit{Burst HDR Datasets}} \\
\midrule
Burst-HDR+ \cite{hasinoff2016burst} & 3750 & 2-10 & Indoor/outdoor, day/night & 80\% \\
Kalantari et al. \cite{kalantari2017deep} & 222 & 3 & Indoor/outdoor, person, motion & 90\% \\
\midrule
\multicolumn{5}{l}{\textit{Non-Burst HDR Datasets}} \\
\midrule
HDM-HDR \cite{froehlich2014creating} & 423 & N/A & Outdoor, Night, extreme bright/dark & 90\% \\
Zurich Raw \cite{ignatov2020replacing} & 504 & N/A & Outdoor driving & 85\% \\
\midrule
\multicolumn{5}{l}{\textit{Non-Burst Image Datasets}} \\
\midrule
Flickr2K & 2650 & N/A & General scenes & 70\% \\
Div2K \cite{Agustsson_2017_CVPR_Workshops} & 800 & N/A & General scenes & 70\% \\
Liu4K \cite{Liu4K} & 1600 & N/A & Ultra high-res scenes & 70\% \\
\midrule
\multicolumn{5}{l}{\textit{Real metalens images (for unsupervised finetuning)}} \\
\midrule
MetaHDR & 200 & 5-20 & Indoor/outdoor, dark/bright, direct illumination/shade & 100\% \\
\bottomrule
\end{tabular}
\label{table:data}
\end{table}
\subsection{Additional dataset details} 
\label{sec:dataset_descp}
\textbf{Synthetic OLED dataset} Our synthetic indoor dataset includes aligned ground truth and low-quality images for burst and non-burst datasets (\cref{table:data}). We simulate artificial hand shake during capture using the pipeline from \cite{brooks2019unprocessing}, adding minor misalignment to training bursts relative to reference frames. The restoration network trains on this synthetic burst data.

\textbf{Real dataset} Our real outdoor dataset for self-supervised finetuning contains unaligned image pairs captured with a compound optic camera. We include diverse scenes spanning daylight, nighttime, and directly illuminated objects (\cref{table:data}). Burst images are first aligned using our training-free alignment module, then fused in the restoration network.

% \subsection{Burst Alignment Quality Assessment}
% \deb{add more details} 

% \input{tables/table_ablation}

\subsection{Extended ablations analysis}

We provide detailed analysis of our ablation studies to justify key design decisions in our framework.

\textbf{Burst Size Analysis.} Ablation results in Table 4 (main paper) shows that increasing burst frames from 3 to 5 provides consistent improvements (26.5 → 26.9 dB PSNR, 0.25 → 0.24 LPIPS). The performance gain plateaus at 5 frames, suggesting this represents the optimal trade-off between information aggregation and motion-induced artifacts. 

\textbf{Model Architecture Choices.} Channel depth analysis reveals that 20 channels provide the optimal capacity, with further increases to 24 channels showing minimal gains (26.5 vs 26.3 dB). Similarly, increasing transformer blocks per Attention-based Fusion Block (AFB) beyond 2 units yields diminishing returns, validating our architectural efficiency. These results demonstrate that our model achieves strong performance without excessive parameterization.

 \begin{figure*}[t]
    \centering
    \includegraphics[width=\linewidth]{figures/assets/fig2_rebut_wacv_lsat.pdf}
    \caption{\textit{Significance of real-world adaptation.} Our model trained just on the synthetic dataset performs poorly in HDR scenes in the real world visualized by the incorrect burst fusion maps. We refine them through unsupervised finetuning using saturation maps computed directly from the real burst  frames leading to higher quality fusion maps. 
    }
    \label{fig:rebut_lsat}
    % \vspace{-2mm}
\end{figure*}
\textbf{Efficacy of $L_{sat}$ in fine-tuning:} We analyze the importance of real-world adaptation in \cref{fig:rebut_lsat}, which improves burst fusion map quality. Initially, due to dynamic range differences between OLED and real-world illumination, the model incorrectly weights contributions from low and high exposed frames, producing poor fusion maps with halo artifacts around bright saturated regions. Our unsupervised fine-tuning with saturation masks corrects these fusion maps, yielding both qualitative and quantitative improvements (NIQE: 7.78 → 5.43, BRISQUE: 31.04 → 23.75).

 \begin{figure*}[t]
    \centering
    \includegraphics[width=\linewidth]{figures/assets/fig_rebut1_1_align2.pdf}
    \caption{\textit{Restoration with mis-alignment.} Our restoration network performs well in the case of moderately misaligned bursts (LoFTR \cite{sun2021loftrdetectorfreelocalfeature}, second row) while leads to slight blurring in case of higher misalignment (HDR+ \cite{hasinoff2016burst}, third row). On the other hand, precise alignment using our proposed alignment module (first row) leads to sharper image features.  
    }
    \label{fig:rebut_align}
    % \vspace{-2mm}
\end{figure*}

\textbf{Impact of alignment errors on restoration quality:} As described in \cref{sec:dataset_descp} our synthetic dataset involves bursts with small artificially introduced shifts. This enables our feature alignment module to spatially align the bursts using the scale-shift feature transform (SFT) layer. In \cref{fig:rebut_align} we visualize the quality of restoration with burst alignment methods which perform inferior to ours and observe that the image quality degrades only slightly when the input burst is not precisely aligned. Specifically, we pair our restoration network with other methods such as LoFTR \cite{sun2021loftrdetectorfreelocalfeature} and HDR+ \cite{hasinoff2016burst} and observe the metrics drop slightly when evaluated over our MetaHDR benchmark:

\vspace{-7pt}
\begin{table}[h]
\centering
\setlength{\aboverulesep}{0pt}
\setlength{\belowrulesep}{0pt}
\setlength{\intextsep}{0pt}
\setlength{\abovecaptionskip}{0pt}
\setlength{\belowcaptionskip}{0pt}
\setlength{\skip\footins}{0pt}
% \setlength\extrarowheight{-4pt}
% \begin{adjustbox}{width=0.85\columnwidth,center}
\begin{threeparttable}
% \caption*{}
\begin{tabular}{@{}ccccc@{}}
\toprule
Method & PSNR \uparrow & SSIM \uparrow & LPIPS \downarrow & NIQE \downarrow \\
\midrule
LoFTR & 26.2 & 0.74 & 0.29 & 5.7 \\[-1pt]
HDR+ & 25.8 & 0.69 & 0.35 & 6.1 \\[-1pt]
Ours & 27.5 & 0.81 & 0.23 & 5.4 \\[-1pt]
\bottomrule
\end{tabular}
% \begin{tablenotes}[flushleft]
% \small
% \item[1] Inference times is average per batch size of 4.
% \item[2] Epochs reported only for training all-in-one models not including prior works.
% \item[3] AutoDIR was trained in 3 stages with the final model used in our evaluations.
% \end{tablenotes}
\end{threeparttable}
% \end{adjustbox}
\end{table}
\vspace{-7pt}
\noindent

\textbf{Component Importance Analysis.} The restoration module ($I_{\text{res}}$) emerges as the most critical component, with its removal causing the largest performance drop (26.5 → 19.9 dB). This substantial degradation highlights the importance of dedicated restoration processing beyond simple feature aggregation. The APCU and AFB modules show comparable importance, with individual removal reducing performance to 24.7 and 24.4 dB respectively. When both are disabled simultaneously, performance drops further to 24.2 dB, indicating some complementary effects between these components.

\textbf{Failure Case Analysis.} Extended burst sequences can suffer from accumulated alignment errors, particularly in scenes with complex motion patterns or significant camera shake. Our analysis in Figure 13.a (main paper) shows that performance degradation typically occurs when motion exceeds the effective receptive field of our alignment module, suggesting potential areas for future improvement through more robust motion modeling. Secondly, although our average capture time per frame is relatively short (20 - 50 ms), fast moving regions such as hands or fingers may appear blurred due to incorrect fusion as visible in Figure 10 (main paper). On the other hand, such blurs might also act as useful indicators of scene motion presence up to a certain threshold.

\setlength{\tabcolsep}{1.5pt}

\begin{figure*}[ht!]
\begin{center}
\small
\begin{tabular}{ccccc}
% \vspace{-0.4mm}
Input &  ADNet &  DRMI &  ESRGAN & HCDeblur  \\[0.5ex]
%\small{Input RGB-D}  &\small{Ours (2 mm)} & \small{Ours (3 mm)} &\small{Ours (4 mm)} & \small{TensorHolo v1} \\
% \raisebox{1.05\height}{\rotatebox{90}{\textbf{Far Focus}}}
%\includegraphics[width=0.3cm]{arrow2.pdf}
\raisebox{0pt}[\height][0pt]{\includegraphics[width=3.2cm]{images/comparison/figure_input_19.pdf}}
&\includegraphics[width=3.2cm]{images/comparison/mag_19_adnet.jpg}
&\includegraphics[width=3.2cm]{images/comparison/mag_19_drmi.jpg}
&\includegraphics[width=3.2cm]{images/comparison/mag_19_esrgan.jpg} 
&\includegraphics[width=3.2cm]{images/comparison/mag_19_hcdeblur.jpg} 
\\[0.5ex]
% & \textbf{Ours (2mm Pupil)} & \textbf{Ours (3mm Pupil)} & \textbf{Ours (4mm Pupil)} & \textbf{Shi et al. 2021}  & \textbf{Shi et al. }  \\[0.5ex]
Ground Truth &  HDRUNet &  NAFNet &  USRNet & Ours  \\[0.5ex]
\includegraphics[width=3.2cm]{images/comparison/mag_19_gt.jpg}
&\includegraphics[width=3.2cm]{images/comparison/mag_19_hdrunet.jpg}
&\includegraphics[width=3.2cm]{images/comparison/mag_19_nafnet.jpg}
&\includegraphics[width=3.2cm]{images/comparison/mag_19_usrnet.jpg} 
&\includegraphics[width=3.2cm]{images/comparison/mag_19_ours-nogan.jpg} 
\\
Input &  ADNet &  DRMI &  ESRGAN & HCDeblur  \\[0.5ex]
%\small{Input RGB-D}  &\small{Ours (2 mm)} & \small{Ours (3 mm)} &\small{Ours (4 mm)} & \small{TensorHolo v1} \\
% \raisebox{1.05\height}{\rotatebox{90}{\textbf{Far Focus}}}
%\includegraphics[width=0.3cm]{arrow2.pdf}
\includegraphics[width=3.2cm]{images/comparison/figure_input_21.pdf}
&\includegraphics[width=3.2cm]{images/comparison/mag_21_adnet.jpg}
&\includegraphics[width=3.2cm]{images/comparison/mag_21_drmi.jpg}
&\includegraphics[width=3.2cm]{images/comparison/mag_21_esrgan.jpg} 
&\includegraphics[width=3.2cm]{images/comparison/mag_21_hcdeblur.jpg} 
\\[0.5ex]
% & \textbf{Ours (2mm Pupil)} & \textbf{Ours (3mm Pupil)} & \textbf{Ours (4mm Pupil)} & \textbf{Shi et al. 2021}  & \textbf{Shi et al. }  \\[0.5ex]
Ground Truth &  HDRUNet &  NAFNet &  USRNet & Ours  \\[0.5ex]
\includegraphics[width=3.2cm]{images/comparison/mag_21_gt.jpg}
&\includegraphics[width=3.2cm]{images/comparison/mag_21_hdrunet.jpg}
&\includegraphics[width=3.2cm]{images/comparison/mag_21_nafnet.jpg}
&\includegraphics[width=3.2cm]{images/comparison/mag_21_usrnet.jpg} 
&\includegraphics[width=3.2cm]{images/comparison/mag_21_ours-nogan.jpg}

 % \vspace{-2mm}
\end{tabular}
\end{center}
\caption{Visual comparisons for different restoration models evaluated on OLED data}
\label{figure:comp_1080}
\end{figure*}
