# Supplementary material for: Enabling High-Quality In-the-Wild Imaging from Severely Aberrated Metalens Bursts
Source: arXiv:2510.10083 source file (2025-10-11)
Supplement: Supplementary file 3 [file oled_supp.tex]

\setlength{\tabcolsep}{1.5pt}

\begin{figure*}[ht!]
\begin{center}
\small
\begin{tabular}{ccccc}
% \vspace{-0.4mm}
Input &  ADNet &  DRMI &  ESRGAN & HCDeblur  \\[0.5ex]
%\small{Input RGB-D}  &\small{Ours (2 mm)} & \small{Ours (3 mm)} &\small{Ours (4 mm)} & \small{TensorHolo v1} \\
% \raisebox{1.05\height}{\rotatebox{90}{\textbf{Far Focus}}}
%\includegraphics[width=0.3cm]{arrow2.pdf}
\raisebox{0pt}[\height][0pt]{\includegraphics[width=3.2cm]{images/comparison/figure_input_19.pdf}}
&\includegraphics[width=3.2cm]{images/comparison/mag_19_adnet.jpg}
&\includegraphics[width=3.2cm]{images/comparison/mag_19_drmi.jpg}
&\includegraphics[width=3.2cm]{images/comparison/mag_19_esrgan.jpg} 
&\includegraphics[width=3.2cm]{images/comparison/mag_19_hcdeblur.jpg} 
\\[0.5ex]
% & \textbf{Ours (2mm Pupil)} & \textbf{Ours (3mm Pupil)} & \textbf{Ours (4mm Pupil)} & \textbf{Shi et al. 2021}  & \textbf{Shi et al. }  \\[0.5ex]
Ground Truth &  HDRUNet &  NAFNet &  USRNet & Ours  \\[0.5ex]
\includegraphics[width=3.2cm]{images/comparison/mag_19_gt.jpg}
&\includegraphics[width=3.2cm]{images/comparison/mag_19_hdrunet.jpg}
&\includegraphics[width=3.2cm]{images/comparison/mag_19_nafnet.jpg}
&\includegraphics[width=3.2cm]{images/comparison/mag_19_usrnet.jpg} 
&\includegraphics[width=3.2cm]{images/comparison/mag_19_ours-nogan.jpg} 
\\
Input &  ADNet &  DRMI &  ESRGAN & HCDeblur  \\[0.5ex]
%\small{Input RGB-D}  &\small{Ours (2 mm)} & \small{Ours (3 mm)} &\small{Ours (4 mm)} & \small{TensorHolo v1} \\
% \raisebox{1.05\height}{\rotatebox{90}{\textbf{Far Focus}}}
%\includegraphics[width=0.3cm]{arrow2.pdf}
\includegraphics[width=3.2cm]{images/comparison/figure_input_21.pdf}
&\includegraphics[width=3.2cm]{images/comparison/mag_21_adnet.jpg}
&\includegraphics[width=3.2cm]{images/comparison/mag_21_drmi.jpg}
&\includegraphics[width=3.2cm]{images/comparison/mag_21_esrgan.jpg} 
&\includegraphics[width=3.2cm]{images/comparison/mag_21_hcdeblur.jpg} 
\\[0.5ex]
% & \textbf{Ours (2mm Pupil)} & \textbf{Ours (3mm Pupil)} & \textbf{Ours (4mm Pupil)} & \textbf{Shi et al. 2021}  & \textbf{Shi et al. }  \\[0.5ex]
Ground Truth &  HDRUNet &  NAFNet &  USRNet & Ours  \\[0.5ex]
\includegraphics[width=3.2cm]{images/comparison/mag_21_gt.jpg}
&\includegraphics[width=3.2cm]{images/comparison/mag_21_hdrunet.jpg}
&\includegraphics[width=3.2cm]{images/comparison/mag_21_nafnet.jpg}
&\includegraphics[width=3.2cm]{images/comparison/mag_21_usrnet.jpg} 
&\includegraphics[width=3.2cm]{images/comparison/mag_21_ours-nogan.jpg}

 % \vspace{-2mm}
\end{tabular}
\end{center}
\caption{Visual comparisons for different restoration models evaluated on OLED data}
\label{figure:comp_1080}
\end{figure*}
