# Supplementary material for: Enabling High-Quality In-the-Wild Imaging from Severely Aberrated Metalens Bursts
Source: arXiv:2510.10083 source file (2025-10-11)
Supplement: Supplementary file 4 [file burst_algo.tex]

\begin{algorithm}[htbp]  
\small  
\caption{Multi-scale Feature Extraction and Homography Estimation}  
\label{alg:multi_homography_part1}  
\SetAlgoLined  
\KwIn{Burst images $\{I^i\}$, deconvolution parameter $\rho$, weights $\{\lambda_k\}$, pyramid levels $K$}  
\KwOut{Homographies $\{H^k\}$ across scales}  

\For{$k = 2$ \KwTo $K$}{  
    Compute $\widetilde{I}^b_k$ via Tikhonov deconvolution:
    
    \[
    \widetilde{I}^b_k = \mathcal{F}^{-1} \left\{ \frac{\bar{\rho^*}}{\lvert\bar{\rho}^2\rvert + \lambda } \mathcal{F}(\widetilde{I}^b_{k-1} \downarrow_2) \right\}
    \]
    where, $\bar{\rho}$ is the optical transfer function or the Discrete Fourier Transform of the PSF ($\rho$) and $\mathcal{F}$  represents the Fast Fourier operation
}  

\For{$k = K$ \KwTo $1$}{  
    Extract feature correspondences and estimate homography:  
    \[
    H^k = \mathtt{get\_pts}(\widetilde{I}^i_k, \widetilde{I}^{i+1}_k)
    \]  
}  
\end{algorithm}

\begin{algorithm}[htbp]  
\small
\caption{Multi-scale displacement fusion}
% \caption{Compute $\{\vec{V}_p\}_K^i$ from homography $H^K$ and Hierarchical Refinement}  
\label{alg:multi_homography_part2}  
\SetAlgoLined  
\KwIn{Homographies $\{H^k\}$, pyramid levels $K$}  
\KwOut{Displacement maps $\{\vec{V}_p\}_i^b$ (final aligned flow fields)}  

Initialize global displacement from coarsest level:  
\[
\{\vec{V}_p\}_K^i \quad \text{from } H^K
\]  

\For{$k = K-1$ \KwTo $1$}{  
    \For{each patch $p$}{  
        Compute local homography $H_p^k$ and displacement $\{\vec{V}_p\}_k^i$  

        Fix the weight to a constant value:  
        \[
        \omega_p = 0.5 \quad \text{(empirically chosen constant)}
        \]  

        Update displacement via weighted aggregation:  
        \[
        \vec{V_p}_k^i = (1 -\omega_p)\,\mathtt{best}\bigl(\vec{V_p}_k^i, 
        \:\:\:\: \{\vec{V_{p'}}_k^i\}_{p' \in \mathcal{N}(p)}\bigr) + \omega_p \,\vec{V_p}_{k+1}^i
        \]  
    }  
}  
\end{algorithm}
