# Supplementary material for: Enabling High-Quality In-the-Wild Imaging from Severely Aberrated Metalens Bursts
Source: arXiv:2510.10083 source file (2025-10-11)
Supplement: Supplementary file 5 [file dataset.tex]

\section{Real Dataset Capture} 

We capture a collection of 100 burst images in both indoor and outdoor illuminations. The bursts are captured using a handheld setup in broad daylight and also low-light conditions to simulate challenging HDR scenarios. After collection, we align the dataset with our burst alignment algorithm for evaluation. 
