# Supplementary material for: Enabling High-Quality In-the-Wild Imaging from Severely Aberrated Metalens Bursts
Source: arXiv:2510.10083 source file (2025-10-11)
Supplement: Supplementary file 6 [file reference_algo.tex]

\begin{algorithm}[htbp]
\small
\caption{Reference Frame Selection Algorithm}
\label{algo:reference_selection}
\SetAlgoLined
\KwIn{Reference exposure time $\leftarrow$ ISP, burst size $N$}
\KwOut{Reference frame $I_{ref}$}

$t_{ref} \leftarrow$ AutoExposure()\;
Initialize burst set $\mathcal{B} \leftarrow \{\}$\;

\For{$i = 1$ \KwTo $N$}{
    $g_i \leftarrow$ SampleDigitalGain()\;
    $I_i \leftarrow$ Capture($t_{ref}$, $g_i$)\;
    $\mathcal{B} \leftarrow \mathcal{B} \cup \{I_i\}$\;
}

$s_{max} \leftarrow 0$, $I_{ref} \leftarrow \text{null}$\;

\For{each $I_i \in \mathcal{B}$}{
    $G_i \leftarrow$ ExtractGreenChannel($I_i$)\;
    $s_i \leftarrow$ GradientSharpness($G_i$)\;
    \If{$s_i > s_{max}$}{
        $s_{max} \leftarrow s_i$, $I_{ref} \leftarrow I_i$\;
    }
}
\Return $I_{ref}$\;
\end{algorithm}
